# Supplementary material for: Emora: An Inquisitive Social Chatbot Who Cares For You
Source: arXiv:2009.04617 source file (2020-09-10)
Supplement: Supplementary file 1 [file appendix.tex]

% \appendix
% \section{Compiled Ontologies}

% Figures \ref{} - \ref{} represent the ontologies compiled and used in the Emora socialbot. All nodes shown in the figures are non-terminals of the ontology, where the final non-terminal layer contains all terminal lexical strings that map to that ontology path. For the sake of figure clarity, the terminal lexical strings are not detailed.

% \begin{figure*}[!htbp]
% \centering
% \includegraphics[width=\textwidth]{figures/ontology_adj.png}
% \caption{} 
% \label{fig:ontadj}
% \end{figure*}

% \begin{figure*}[!htbp]
% \centering
% \includegraphics[width=\textwidth]{figures/ontology_demographics.png}
% \caption{} 
% \label{fig:ontdemog}
% \end{figure*}
